# Supplementary material for: A general approximation lower bound in $L^p$ norm, with applications to feed-forward neural networks
Source: arXiv:2206.04360 source file (2022-12-20)
Supplement: Supplementary file 1 [file newAppendixMendelson.tex]

% Si on décide de donner les détails sur l'extension de Mendelson (suppression de l'hypothèse technique de mesurabilité) :

% Attention, cette section est une v0.

Proposition \ref{result_mendelson} was originally stated by Mendelson \cite[Corollary $3.12$]{971753} when $[a,b] = [0,1]$ and when $G$ is a uniform Glivenko-Cantelli class. However, we prove that the Glivenko-Cantelli assumption is not necessary, and that the result extends to sets of functions in any segment $[a,b]$.

We begin by rewriting the proof of Corollary $3.12$ in \cite{971753}, but without assuming that $G$ is a uniform Glivenko Cantelli class. To this end, we will use the following result from \cite{971753}:

\begin{lemma}[Theorem $3.2$ in \cite{971753}]
  \label{lemma:thm32mendelson}
  Let $G \subset B(L_{\infty}(\mathcal{X}))$, \red{$0 < \varepsilon < 1$}, $n \in \NN^*$ and $p \geq 1$. There exists a constant $c$ depending only on $p$ such that for every empirical measure $\mu_n > 0$,
  $$
  \log M\left(\varepsilon, G, \|\cdot\|_{L^p(\mu_n)}\right) \leq c \fat_{\frac{\varepsilon}{8}}(G) \log^2 \left(\frac{2 \fat_{\frac{\varepsilon}{8}}(G)}{\varepsilon}\right).
  $$
\end{lemma}

\begin{proof}[Proof (rewriting of the proof of Corollary $3.12$ in \cite{971753})]
Let \red{$0 <\varepsilon < 1$}. Consider $\{f_1, \ldots, f_m\} \subset G$ an $\varepsilon$-packing of $G$ in $L^p(\mu)$ with finite cardinal $m$. Let $\varepsilon'~:=~\min_{i \neq j} \|f_i~-~f_j\|_{L^p(\mu)}$ and let $\delta := \varepsilon' - \varepsilon$. By definition of an $\varepsilon$-packing, it holds that $\varepsilon' > \varepsilon$ and thus $\delta > 0$. We are going to prove that there exist an integer $n \geq 1$ and an empirical measure $\mu_n$ such that $\{f_1, \ldots, f_m\}$ is also an $\varepsilon$-packing of $G$ in $L^p(\mu_n)$. Fix $n \geq 1$ and let $X_1, \ldots, X_n$ be $n$ independent random variables with same distribution $\mu$. We denote by $\mu_n$ the empirical distribution with support $\{X_1, \ldots, X_n\}$. Note that we have
\begin{multline}
    \label{eq:empirical_measure}
    \PROBA \left( \exists i \neq j, \ \|f_i - f_j\|_{L^p(\mu_n)} \leq \|f_i - f_j\|_{L^p(\mu)} - \delta \right) \\ 
    \leq \sum_{1 \leq i < j \leq m} \PROBA \left( \|f_i - f_j\|^p_{L^p(\mu_n)} \leq \|f_i - f_j\|^p_{L^p(\mu)} - \delta^p \right).
"\end{multline}
For fixed $i, j$, let $Z^{i,j}_k = |f_i(X_k) - f_j(X_k)|^p$, $k=1, \ldots, n$. These random variables have same distribution, with values in $[0,1]$ and are independent since the $X_k$ are. Note that $\|f_i - f_j\|^p_{L^p(\mu_n)}$ writes as $\frac{1}{n} \sum_{k=1}^n Z^{i,j}_k$, and has mathematical expectation $\|f_i - f_j\|_{L^p(\mu)}$ (with respect to $\mu$). We can thus rewrite \eqref{eq:empirical_measure} as
\begin{align*}
\PROBA \left( \exists i \neq j, \ \|f_i - f_j\|_{L^p(\mu_n)} \leq \|f_i - f_j\|_{L^p(\mu)} - \delta \right)
&\leq \frac{m(m-1)}{2} \max_{i \neq j} \PROBA \left( \sum_{k=1}^n Z^{i,j}_k - n\mathbb{E}_{\mu}Z^{i,j}_1 \leq - n\delta^p \right) \\
&\leq \frac{m(m-1)}{2} \exp \left( -2 n \delta^{2p} \right),
\end{align*}
where in the second line, we applied the Hoeffding inequality. It is thus sufficient to select $n~=~\left\lceil \frac{1}{2 \delta^{2p}} \log\left( \frac{m(m-1)}{2} \right) \right\rceil + 1$ to have that the left hand side above is strictly less than $1$. We have found that there exist $n \in \NN$ and an empirical measure $\mu_n$ such that for all $i \neq j$, $\|f_i - f_j\|_{L^p(\mu_n)} > \|f_i - f_j\|_{L^p(\mu)} - \delta \geq \varepsilon' - \delta = \varepsilon$. It follows that $\{f_1, \ldots, f_m\}$ is an $\varepsilon$-packing in $L^p(\mu_n)$, which entails
\begin{align*}
    M\left( \varepsilon, G, \|\cdot\|_{L^p(\mu)} \right) \leq M\left( \varepsilon, G, \|\cdot\|_{L^p(\mu_n)} \right).
\end{align*}
The result follows from Lemma \ref{lemma:thm32mendelson}.
\end{proof}

We now explain how to derive Proposition~\ref{result_mendelson} (with an arbitrary range $[a,b]$) as a straightforward consequence of Corollary $3.12$ in \cite{971753}.

\begin{proof}[Proof (of Proposition \ref{result_mendelson}).]
\label{proof_lemma_ext_mendel}
In order to apply Proposition~\ref{prop_mendelson_original}, we reduce the problem from $[a,b]$ to $[0,1]$ by translating and rescaling every function in $G$. For $g \in G$, we define $\tilde{g}:\cX \to [0,1]$ by $\tilde{g}(x) = \frac{g(x) - a}{b-a}$, and we set
$$
\tilde{G} = \left\{\tilde{g} \; : \ g \in G \right\} \;.
$$
Note that every $\tilde{g} \in \tilde{G}$ is indeed $[0,1]$-valued.

We now note that translation does not affect packing numbers nor the fat-shattering dimension, while rescaling only changes the scale $\eps$ by a factor of $b-a$. More precisely, we have the following two properties:

\textbf{Property 1:} For all $u > 0$, $\fat_{\frac{u}{b-a}}(\tilde{G}) = \fat_u(G)$. \\
\textbf{Property 2:} For all $u > 0$, $M\!\left(\frac{u}{b-a}, \tilde{G}, \|\cdot\|_{L^p(\mu)}\right) = M\!\left(u, G, \|\cdot\|_{L^p(\mu)}\right)$.

Before proving the two properties (see below), we first conclude the proof of Proposition \ref{result_mendelson}. By Property~1, $\fat_{\gamma}(\tilde{G}) = \fat_{\gamma (b-a)}(G)$, which by assumption is finite for all $\gamma>0$. Since every $\tilde{g} \in \tilde{G}$ is $[0,1]$-valued, we can thus apply Proposition~\ref{prop_mendelson_original}. Using it with $\tilde{\eps} = \eps/(b-a)$, we get
\[
\log M\!\left(\tilde{\varepsilon}, \tilde{G}, \|\cdot\|_{L^p(\mu)}\right) \leq c_p \fat_{\frac{\tilde{\varepsilon}}{8}}(\tilde{G}) \log^2 \!\left(\frac{2 \fat_{\frac{\tilde{\varepsilon}}{8}}(\tilde{G})}{\tilde{\varepsilon}}\right) \;.
\]
Combining with the two equalities in Properties~1 and ~2, we obtain
\[
\log M\!\left(\eps, G, \|\cdot\|_{L^p(\mu)}\right) \leq c_p \fat_{\frac{\eps}{8}}(G) \log^2 \!\left(\frac{2 (b-a) \fat_{\frac{\eps}{8}}(G)}{\eps}\right) \;,
\]
which concludes the proof of Proposition \ref{result_mendelson}.

We now prove the two properties.

\textbf{Proof of Property~1.} We first show that $\fat_{\frac{u}{b-a}}(\tilde{G}) \geq \fat_u(G)$. To that end, let $S = \{x_1, \ldots, x_m\}$ and $r : S \to \mathbb{R}$ be such that for any $E \subset S$, there exists $g \in G$ such that \red{$g(x) \geq r(x) + u$} if $x \in E$ and \red{$g(x) \leq r(x) - u$} otherwise. Setting $\tilde{r}(x) = \frac{r(x) - a}{b-a}$, we can see that \red{$\tilde{g}(x) \geq \tilde{r}(x) + \frac{u}{b-a}$} if $x \in E$ and \red{$\tilde{g}(x) \leq \tilde{r}(x) - \frac{u}{b-a}$} otherwise, which proves $\fat_{\frac{u}{b-a}}(\tilde{G}) \geq \fat_u(G)$. The reverse inequality is proved similarly.

\textbf{Proof of Property~2.} Let $\{g_1, \ldots, g_m\}$ be a $u$-packing of $G$ in $L^p(\mu)$ norm. This means that $\|g_i - g_j\|_{L^p(\mu)}>u$ and therefore $\|\tilde{g}_i - \tilde{g}_j\|_{L^p(\mu)}>\frac{u}{b-a}$ for all $i \neq j \in \{1,\ldots,m\}$, so that $\{\tilde{g}_1, \ldots, \tilde{g}_m\} \subset \tilde{G}$ is a $\frac{u}{b-a}$-packing of $\tilde{G}$. This proves $M\bigl(\frac{u}{b-a}, \tilde{G}, \|\cdot\|_{L^p(\mu)}\bigr) \geq M\bigl(u, G, \|\cdot\|_{L^p(\mu)}\bigr)$.
The reverse inequality is proved similarly.
\end{proof}
